# Supplementary material for: The cooperation-defection evolution on social networks
Source: arXiv:2007.09856 source file (2021-09-15)
Supplement: Supplementary file 1 [file Supplementary_material_arxiv_.pdf]

# Supplementary Material: The cooperation-defection evolution on social networks

Bijan Sarkar

## Contents

|     |                                                                 |   |
|-----|-----------------------------------------------------------------|---|
| 1   | Ground environment: the underlying interaction nature . . . . . | 1 |
| 2   | Outcomes of the dynamical system . . . . .                      | 2 |
| 2.1 | Base matrix game . . . . .                                      | 3 |
| 2.2 | Prisoner's dilemma game . . . . .                               | 4 |
| 2.3 | Snowdrift game . . . . .                                        | 4 |
| 2.4 | Stag-hunt game . . . . .                                        | 5 |
| 3   | Summary notes . . . . .                                         | 6 |
|     | Reference . . . . .                                             | 6 |

## 1 Ground environment: the underlying interaction nature

If the payoffs of an  $i^{th}$  individual getting from an interaction with a  $j^{th}$  individual are denoted by the  $\pi_{ij}$ , then in general the base payoff matrix for the cooperation-defection interaction is given by:  $\pi_{CC} = b - c$ ,  $\pi_{CD} = -c$ ,  $\pi_{DC} = b$ ,  $\pi_{DD} = 0$ , where cooperators pay cost  $c > 0$  to provide a benefit  $b > c$ . Defectors neither pay cost nor contribute benefit. Besides this payoff matrix, on the well-known three game classes, namely Dominance game, Coexistence game and Coordination game, other cooperation-defection payoff matrices can also be defined to encompass general social dilemmas between cooperators and defectors where the general behavioural character of cooperator and defector is inherently incorporated with each of the games in the sense that in the intratype competition, the cooperator payoff is higher

than the defector payoff ( $\pi_{CC} > \pi_{DD}$ ), on the contrary in the intertype competition a defector gains higher payoff than a cooperator ( $\pi_{DC} > \pi_{CD}$ ), and to get a higher payoff each type of individuals prefers to interact with a cooperator than a defector ( $\pi_{CC} > \pi_{CD}$  and  $\pi_{DC} > \pi_{DD}$ ). By this concept each of the payoff values for various well-known games is bounded into more restricted ways under the three game classes. However, it will be important to note that the occurrence of an expected recognised character of a specific game which is operated by the mathematical inequalities of the payoffs of the social dilemmas is highly influenced by the number of presence individuals of the evolutionary system.

## 2 Outcomes of the dynamical system

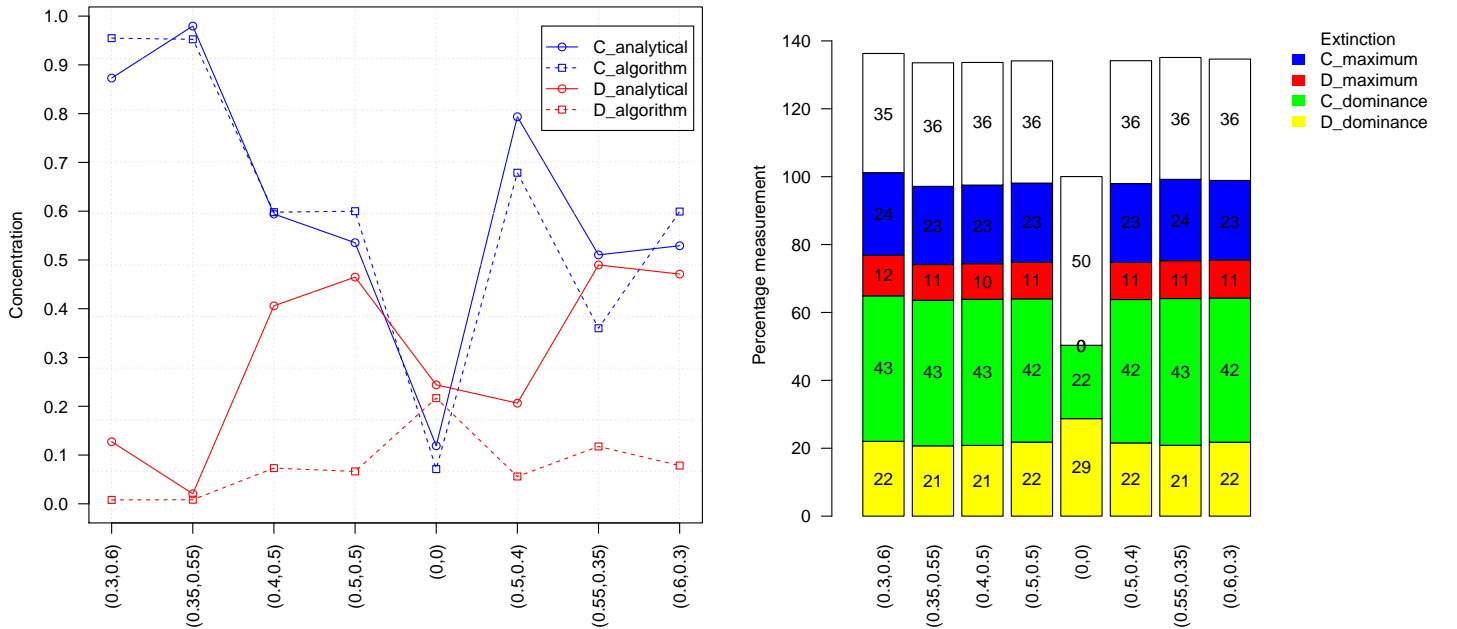

Fig. S.1: Base matrix game: The outcomes after 20,000 time steps with a generation interval of 0.002 time scale are examined provided the number of allocable vertices and the degree of the graph being 100 and 5, respectively.

## 2.1 Base matrix game

In what extent the evolutionary process having significantly been influenced by total number of individuals is prominently notice in Fig. S.1 at the absence of random drift. One can conclude here that the total number of individuals controls the rate of evolution. Another base matrix game is examined in the consideration of fitness payoffs:  $\pi_{CC} = 1.5$ ,  $\pi_{CD} = -0.7$ ,  $\pi_{DC} = 2.2$ ,  $\pi_{DD} = 0.5$ , where the random drift coefficient set to  $0.5 \times 10^{-1}$  in the algorithm method. For  $\mathcal{N} = 100$ , observable values with and without random drift respectively are:  $38 \leq \text{C\_dominance} \leq 40$ ,  $23 \leq \text{D\_dominance} \leq 25$  and  $\text{C\_dominance} = 12$ ,  $\text{D\_dominance} = 17$  while for  $\mathcal{N} = 1000$ :  $39 \leq \text{C\_dominance} \leq 40$ ,  $23 \leq \text{D\_dominance} \leq 24$  and  $\text{C\_dominance} = 13$ ,  $\text{D\_dominance} = 0$ .

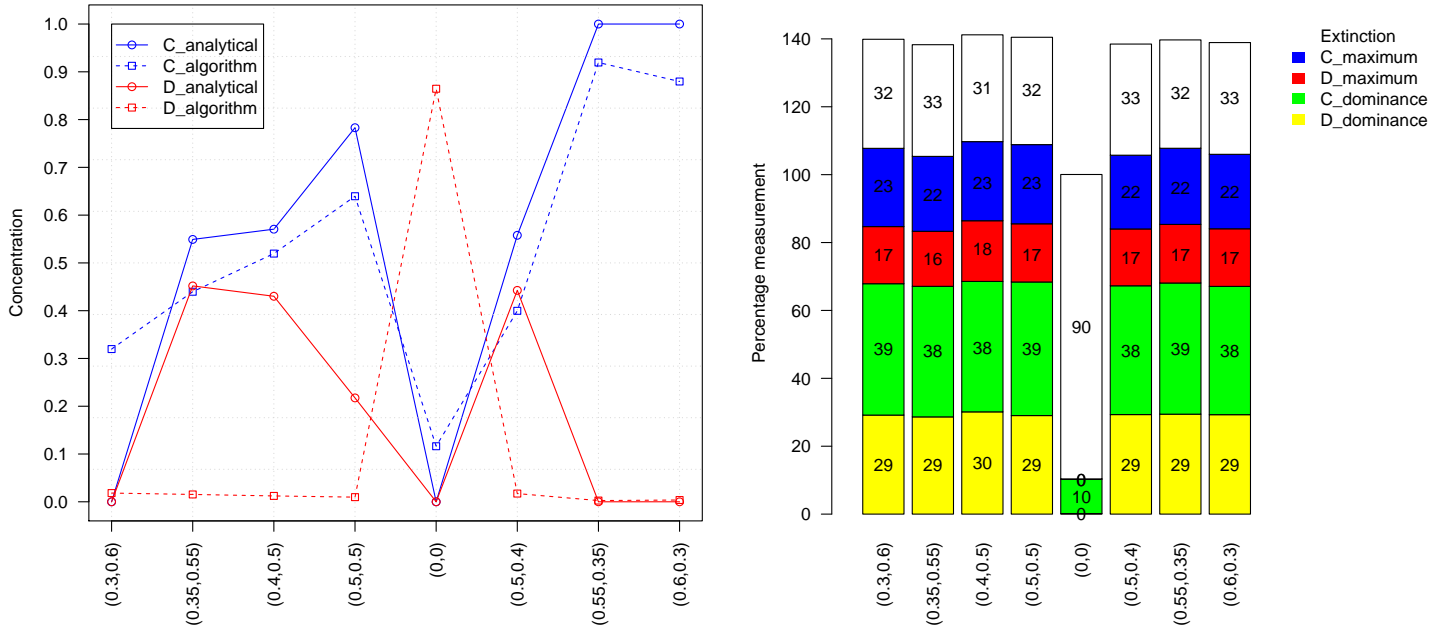

Fig. S.2: Prisoner's dilemma game: The outcomes after 20,000 time steps with a generation interval of 0.02 time scale are examined in the consideration of maximum fitness, 1.145, and of fitness payoffs:  $\pi_{CC} = 1.5$ ,  $\pi_{CD} = 0.3$ ,  $\pi_{DC} = 2.2$ ,  $\pi_{DD} = 0.5$ . The number of allocable vertices and the degree of the graph respectively are 1000 and 50 where the random drift coefficient in the analytical procedure and the algorithm method respectively is  $10^{-5}$  and  $0.5 \times 10^{-1}$ .

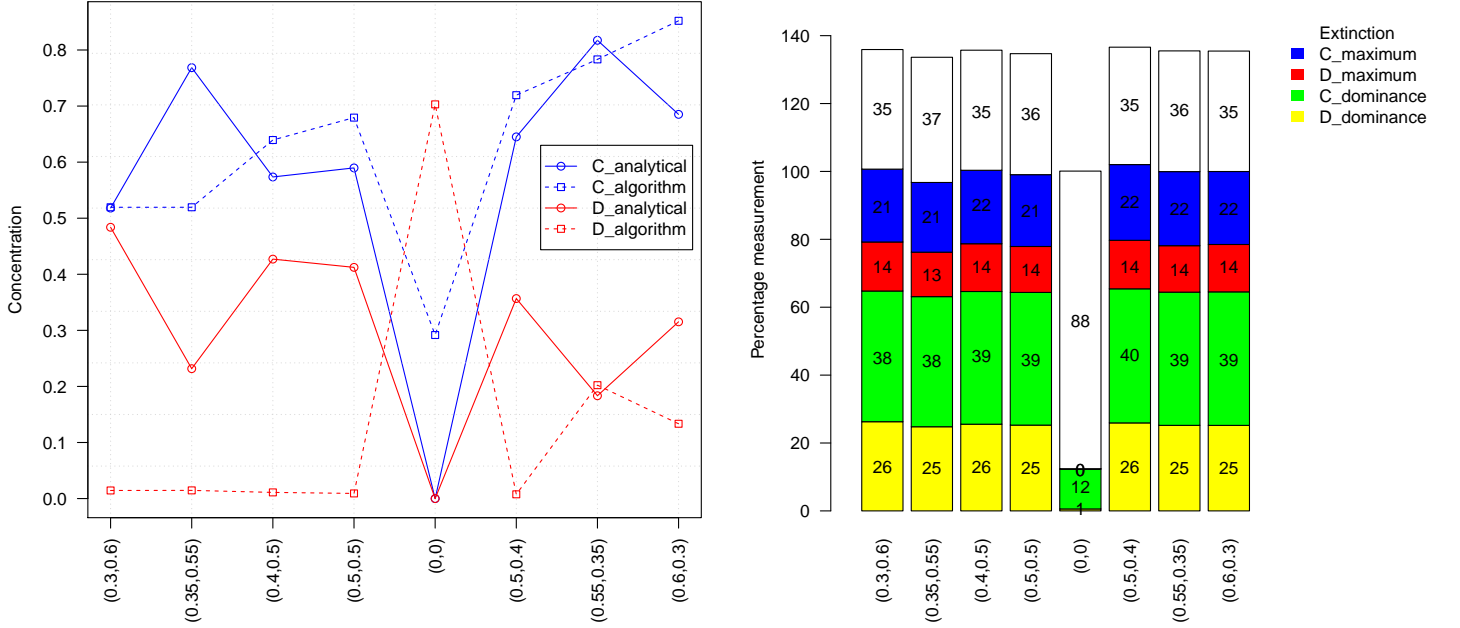

Fig. S.3: Snowdrift game: The outcomes after 20,000 time steps with a generation interval of 0.02 time scale are examined in the consideration of maximum fitness, 1.145, and of fitness payoffs:  $\pi_{CC} = 1.5$ ,  $\pi_{CD} = 0.5$ ,  $\pi_{DC} = 2.2$ ,  $\pi_{DD} = 0.3$ . The number of allocable vertices and the degree of the graph respectively are 1000 and 50 where the random drift coefficient in the analytical procedure and the algorithm method respectively is  $10^{-5}$  and  $0.5 \times 10^{-1}$ .

## 2.2 Prisoner's dilemma game

Prisoner's dilemma game is an example of D-dominance game class of very minimum defector fitness payoff in intratype competition, see Fig. S.2. For  $\mathcal{N} = 100$ , observable values with and without random drift respectively are:  $38 \leq \text{C\_dominance} \leq 39$ ,  $29 \leq \text{D\_dominance} \leq 31$  and  $\text{C\_dominance} = 14$ ,  $\text{D\_dominance} = 54$ .

## 2.3 Snowdrift game

Snowdrift game is an example of coexistence game class of relatively high defector fitness payoff in intertype competition, see Fig. S.3. For  $\mathcal{N} = 100$ , observable values with and without random drift respectively are:  $39 \leq \text{C\_dominance} \leq 40$ ,  $25 \leq$

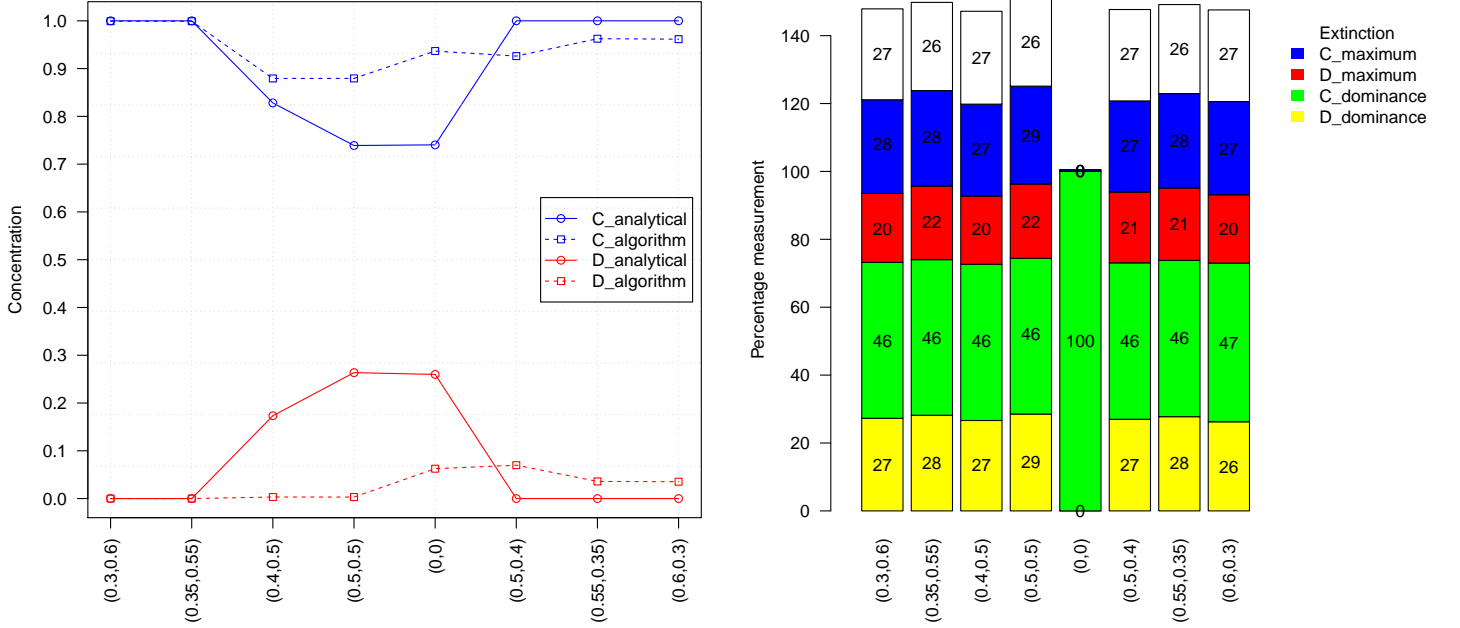

Fig. S.4: Stag-hunt game: The outcomes after 20,000 time steps with a generation interval of 0.02 time scale are examined in the consideration of maximum fitness, 1.145, and of fitness payoffs:  $\pi_{CC} = 2.2$ ,  $\pi_{CD} = 0.3$ ,  $\pi_{DC} = 1.5$ ,  $\pi_{DD} = 0.5$ . The number of allocable vertices and the degree of the graph respectively are 1000 and 50 where the random drift coefficient in the analytical procedure and the algorithm method respectively is  $10^{-5}$  and  $0.3 \times 10^{-1}$ .

D\_dominance  $\leq 26$  and C\_dominance = 20, D\_dominance = 54.

## 2.4 Stag-hunt game

Stag-hunt game is an example of coordination game class of relatively high cooperator fitness payoff in intratype competition, see Fig. S.4. For  $\mathcal{N} = 100$ , observable values with and without random drift respectively are:  $46 \leq \text{C\_dominance} \leq 47$ ,  $27 \leq \text{D\_dominance} \leq 29$  and C\_dominance = 100, D\_dominance = 0.

### 3 Summary notes

- The evolution is the consequence of gene variation.
- One of the factors for the gene variation is the fitness of the individual which is the combination of the fertility parameter and the viability parameter [S.1].
- The gene variation also occurs due to the random drift effect.
- The random drift is the result of the random change in physiological pattern, social behaviour, ecology, etc. Thus, determination of the specific reason for the random drift can be difficult.
- In the course of cooperation enhancement in the long run of the evolutionary process, the random drift helps to flourish the intratype fitness character of cooperators . Of particular note is the random drift sustaining the environment of biodiversity.
- In the absence of the cooperators the defectors will extinct.
- The dominant character of cooperation over defection generally remains unaffected on any environmental circumstances.
- It is understandable that the evolutionary factors are somehow dependent on each other.

### Reference

- [S.1] M.E. Scott, D.M. Scott, E. Pollak, Conditions under which the mean fertility is maximized when a population is at a stable equilibrium, *Genetics* 118(4)1988 713 – 720.
